# Supplementary material for: Combined measurement of velocity and temperature in liquid metal convection
Source: arXiv:1907.03472 ancillary file (2020-02-18)
Supplement: Supplementary file 1 [file Supplement_data_table.pdf]

Supplementary material for the article *Combined measurement of velocity and temperature in liquid metal convection* by Till Zürner, Felix Schindler, Tobias Vogt, Sven Eckert and Jörg Schumacher.

The table below shows selected experimental data presented in figures 5, 8 and 9 of the article. Uncertainties of the quantities are given as standard deviation. The uncertainty of the Prandtl number $Pr$ is at most 0.0001 for $Ra > 5 \times 10^7$. The time series of measurements marked with † are shown in figures 3 and 4. More details on the definition of the listed quantities can be found in the article.

| | $Ra$ | $Pr$ | $f_{osc}/f_\kappa$ | $f_{to}/f_\kappa$ | $Re_{LSC}$ | $Re_{vert}$ | $Re_{centre}$ | $Nu$ |
|---|---|---|---|---|---|---|---|---|
| † | $(9.68 \pm 0.37) \times 10^5$ | 0.0292 | $27.3 \pm 2.8$ | $26.1 \pm 4.4$ | $(2.87 \pm 0.43) \times 10^3$ | $(2.78 \pm 0.60) \times 10^3$ | $(1.47 \pm 0.48) \times 10^3$ | – |
| | $(9.88 \pm 0.33) \times 10^5$ | 0.0292 | $28.3 \pm 1.6$ | $24.9 \pm 3.7$ | $(2.73 \pm 0.37) \times 10^3$ | $(2.57 \pm 1.02) \times 10^3$ | $(1.62 \pm 0.43) \times 10^3$ | – |
| | $(1.01 \pm 0.04) \times 10^6$ | 0.0292 | $28.4 \pm 3.5$ | $26.1 \pm 4.3$ | $(2.87 \pm 0.43) \times 10^3$ | $(2.88 \pm 0.62) \times 10^3$ | $(1.54 \pm 0.50) \times 10^3$ | – |
| | $(1.04 \pm 0.03) \times 10^6$ | 0.0292 | $27.8 \pm 3.1$ | $25.0 \pm 4.1$ | $(2.76 \pm 0.42) \times 10^3$ | $(3.37 \pm 0.80) \times 10^3$ | $(1.76 \pm 0.43) \times 10^3$ | – |
| | $(1.04 \pm 0.04) \times 10^6$ | 0.0292 | $30.1 \pm 0.9$ | $26.5 \pm 4.0$ | $(2.91 \pm 0.40) \times 10^3$ | $(2.83 \pm 0.69) \times 10^3$ | $(1.50 \pm 0.41) \times 10^3$ | – |
| | $(1.05 \pm 0.02) \times 10^6$ | 0.0292 | $29.5 \pm 1.7$ | $26.3 \pm 4.3$ | $(2.89 \pm 0.43) \times 10^3$ | $(2.90 \pm 0.62) \times 10^3$ | $(1.53 \pm 0.46) \times 10^3$ | – |
| | $(1.11 \pm 0.04) \times 10^6$ | 0.0292 | $27.5 \pm 1.4$ | $28.2 \pm 5.2$ | $(3.13 \pm 0.54) \times 10^3$ | $(3.15 \pm 1.01) \times 10^3$ | $(1.95 \pm 0.54) \times 10^3$ | – |
| | $(1.11 \pm 0.04) \times 10^6$ | 0.0292 | $29.0 \pm 2.3$ | $26.6 \pm 4.3$ | $(2.92 \pm 0.42) \times 10^3$ | $(3.30 \pm 0.87) \times 10^3$ | $(1.77 \pm 0.44) \times 10^3$ | – |
| | $(1.57 \pm 0.05) \times 10^6$ | 0.0292 | $32.9 \pm 4.6$ | $31.0 \pm 4.4$ | $(3.40 \pm 0.45) \times 10^3$ | $(3.95 \pm 0.89) \times 10^3$ | $(2.29 \pm 0.58) \times 10^3$ | – |
| | $(1.60 \pm 0.04) \times 10^6$ | 0.0292 | $32.2 \pm 3.2$ | $30.1 \pm 5.2$ | $(3.32 \pm 0.51) \times 10^3$ | $(3.72 \pm 1.18) \times 10^3$ | $(2.33 \pm 0.51) \times 10^3$ | – |
| | $(1.66 \pm 0.07) \times 10^6$ | 0.0292 | $33.8 \pm 3.5$ | $31.0 \pm 6.2$ | $(3.44 \pm 0.59) \times 10^3$ | $(3.40 \pm 0.84) \times 10^3$ | $(2.02 \pm 0.62) \times 10^3$ | – |
| | $(1.73 \pm 0.06) \times 10^6$ | 0.0292 | $35.4 \pm 4.6$ | $32.3 \pm 6.4$ | $(3.59 \pm 0.60) \times 10^3$ | $(3.67 \pm 0.83) \times 10^3$ | $(2.00 \pm 0.65) \times 10^3$ | – |
| | $(2.01 \pm 0.05) \times 10^6$ | 0.0292 | $35.5 \pm 4.1$ | $33.6 \pm 6.2$ | $(3.71 \pm 0.57) \times 10^3$ | $(4.32 \pm 1.20) \times 10^3$ | $(2.52 \pm 0.61) \times 10^3$ | – |
| | $(2.09 \pm 0.05) \times 10^6$ | 0.0292 | $33.8 \pm 5.6$ | $33.5 \pm 8.0$ | $(3.77 \pm 0.77) \times 10^3$ | $(4.88 \pm 1.25) \times 10^3$ | $(2.61 \pm 0.66) \times 10^3$ | – |
| | $(2.09 \pm 0.08) \times 10^6$ | 0.0292 | $36.9 \pm 5.4$ | $34.4 \pm 6.2$ | $(3.80 \pm 0.60) \times 10^3$ | $(4.23 \pm 1.11) \times 10^3$ | $(2.31 \pm 0.68) \times 10^3$ | – |
| | $(2.13 \pm 0.05) \times 10^6$ | 0.0292 | $36.3 \pm 3.2$ | $33.7 \pm 5.8$ | $(3.71 \pm 0.58) \times 10^3$ | $(4.37 \pm 0.92) \times 10^3$ | $(2.32 \pm 0.67) \times 10^3$ | – |
| | $(2.17 \pm 0.08) \times 10^6$ | 0.0292 | $38.0 \pm 1.5$ | $35.6 \pm 6.3$ | $(3.93 \pm 0.61) \times 10^3$ | $(3.84 \pm 0.89) \times 10^3$ | $(2.15 \pm 0.68) \times 10^3$ | – |
| | $(2.18 \pm 0.05) \times 10^6$ | 0.0292 | $37.0 \pm 5.2$ | $36.6 \pm 8.1$ | $(4.10 \pm 0.79) \times 10^3$ | $(4.28 \pm 1.29) \times 10^3$ | $(2.40 \pm 0.72) \times 10^3$ | – |
| | $(2.27 \pm 0.05) \times 10^6$ | 0.0292 | $37.4 \pm 6.3$ | $34.1 \pm 6.7$ | $(3.79 \pm 0.66) \times 10^3$ | $(4.41 \pm 1.26) \times 10^3$ | $(2.39 \pm 0.81) \times 10^3$ | – |
| | $(2.30 \pm 0.06) \times 10^6$ | 0.0292 | $36.2 \pm 7.2$ | $34.6 \pm 6.2$ | $(3.83 \pm 0.62) \times 10^3$ | $(4.47 \pm 1.03) \times 10^3$ | $(2.56 \pm 0.71) \times 10^3$ | – |
| | $(3.12 \pm 0.07) \times 10^6$ | 0.0292 | $39.9 \pm 7.0$ | $40.7 \pm 7.6$ | $(4.51 \pm 0.76) \times 10^3$ | $(4.64 \pm 1.04) \times 10^3$ | $(2.88 \pm 0.95) \times 10^3$ | – |
| | $(3.12 \pm 0.08) \times 10^6$ | 0.0292 | $43.3 \pm 8.2$ | $37.1 \pm 9.1$ | $(4.20 \pm 0.92) \times 10^3$ | $(5.21 \pm 1.73) \times 10^3$ | $(2.98 \pm 0.83) \times 10^3$ | – |
| | $(3.14 \pm 0.07) \times 10^6$ | 0.0292 | $42.7 \pm 5.5$ | $40.3 \pm 8.8$ | $(4.52 \pm 0.89) \times 10^3$ | $(4.10 \pm 2.15) \times 10^3$ | $(3.14 \pm 0.88) \times 10^3$ | – |
| | $(3.19 \pm 0.09) \times 10^6$ | 0.0292 | $45.4 \pm 1.4$ | $39.1 \pm 9.4$ | $(4.38 \pm 0.78) \times 10^3$ | $(4.27 \pm 1.65) \times 10^3$ | $(2.90 \pm 0.87) \times 10^3$ | – |
| | $(4.10 \pm 0.08) \times 10^6$ | 0.0292 | $44.5 \pm 6.2$ | $43.9 \pm 8.2$ | $(4.86 \pm 0.83) \times 10^3$ | $(5.21 \pm 1.90) \times 10^3$ | $(3.29 \pm 1.07) \times 10^3$ | – |
| | $(4.14 \pm 0.17) \times 10^6$ | 0.0292 | $41.3 \pm 7.0$ | $41.7 \pm 10.7$ | $(4.73 \pm 1.05) \times 10^3$ | $(5.84 \pm 1.40) \times 10^3$ | $(3.75 \pm 0.97) \times 10^3$ | $7.27 \pm 0.76$ |
| | $(4.18 \pm 0.13) \times 10^6$ | 0.0292 | $45.9 \pm 8.6$ | $42.7 \pm 10.7$ | $(4.84 \pm 1.08) \times 10^3$ | $(5.27 \pm 1.56) \times 10^3$ | $(3.29 \pm 1.00) \times 10^3$ | $7.47 \pm 0.81$ |
| | $(4.18 \pm 0.10) \times 10^6$ | 0.0292 | $47.1 \pm 7.4$ | $41.9 \pm 12.8$ | $(4.83 \pm 1.18) \times 10^3$ | $(6.15 \pm 1.41) \times 10^3$ | $(3.26 \pm 0.96) \times 10^3$ | – |
| | $(4.18 \pm 0.15) \times 10^6$ | 0.0292 | $45.5 \pm 5.8$ | $44.6 \pm 12.1$ | $(5.04 \pm 0.97) \times 10^3$ | $(5.07 \pm 1.58) \times 10^3$ | $(2.96 \pm 0.96) \times 10^3$ | – |
| | $(6.28 \pm 0.23) \times 10^6$ | 0.0292 | $57.2 \pm 10.1$ | $52.5 \pm 10.7$ | $(5.85 \pm 1.03) \times 10^3$ | $(6.56 \pm 1.44) \times 10^3$ | $(3.82 \pm 1.17) \times 10^3$ | $8.08 \pm 0.90$ |
| | $(6.34 \pm 0.16) \times 10^6$ | 0.0292 | $55.6 \pm 12.4$ | $53.5 \pm 11.2$ | $(5.96 \pm 1.07) \times 10^3$ | $(6.30 \pm 1.51) \times 10^3$ | $(4.10 \pm 1.27) \times 10^3$ | – |
| | $(6.46 \pm 0.14) \times 10^6$ | 0.0292 | $53.8 \pm 7.2$ | $52.6 \pm 11.2$ | $(5.87 \pm 1.06) \times 10^3$ | $(6.35 \pm 2.38) \times 10^3$ | $(3.99 \pm 1.12) \times 10^3$ | – |
| | $(6.50 \pm 0.19) \times 10^6$ | 0.0292 | $55.7 \pm 8.9$ | $54.5 \pm 11.3$ | $(6.07 \pm 1.07) \times 10^3$ | $(6.78 \pm 1.51) \times 10^3$ | $(3.91 \pm 1.19) \times 10^3$ | $8.19 \pm 0.73$ |

| | $Ra$ | $Pr$ | $f_{\mathrm{osc}}/f_{\kappa}$ | $f_{\mathrm{to}}/f_{\kappa}$ | $Re_{\mathrm{LSC}}$ | $Re_{\mathrm{vert}}$ | $Re_{\mathrm{centre}}$ | $Nu$ |
|---|---|---|---|---|---|---|---|---|
| | $(8.38 \pm 0.23) \times 10^6$ | 0.0292 | $58.6 \pm 8.9$ | $58.3 \pm 13.3$ | $(6.53 \pm 1.23) \times 10^3$ | $(7.57 \pm 2.65) \times 10^3$ | $(4.41 \pm 1.44) \times 10^3$ | – |
| | $(8.68 \pm 0.29) \times 10^6$ | 0.0292 | $62.3 \pm 11.0$ | $59.6 \pm 13.7$ | $(6.67 \pm 1.21) \times 10^3$ | $(7.07 \pm 1.51) \times 10^3$ | $(4.50 \pm 1.40) \times 10^3$ | $8.56 \pm 0.81$ |
| | $(8.80 \pm 0.24) \times 10^6$ | 0.0292 | $60.2 \pm 12.4$ | $60.5 \pm 13.2$ | $(6.77 \pm 1.25) \times 10^3$ | $(7.26 \pm 1.83) \times 10^3$ | $(4.56 \pm 1.34) \times 10^3$ | – |
| | $(9.85 \pm 0.28) \times 10^6$ | 0.0293 | $66.1 \pm 8.0$ | $64.1 \pm 13.4$ | $(7.14 \pm 1.27) \times 10^3$ | $(7.92 \pm 1.78) \times 10^3$ | $(4.83 \pm 1.40) \times 10^3$ | $9.03 \pm 0.65$ |
| | $(1.03 \pm 0.03) \times 10^7$ | 0.0292 | $66.2 \pm 13.1$ | $66.2 \pm 17.8$ | $(7.44 \pm 1.38) \times 10^3$ | $(7.60 \pm 2.22) \times 10^3$ | $(4.86 \pm 1.42) \times 10^3$ | – |
| | $(1.04 \pm 0.02) \times 10^7$ | 0.0292 | $65.7 \pm 11.8$ | $63.0 \pm 13.9$ | $(7.06 \pm 1.37) \times 10^3$ | $(8.03 \pm 2.80) \times 10^3$ | $(5.02 \pm 1.56) \times 10^3$ | – |
| | $(1.04 \pm 0.03) \times 10^7$ | 0.0292 | $65.5 \pm 10.3$ | $64.5 \pm 15.2$ | $(7.24 \pm 1.39) \times 10^3$ | $(7.56 \pm 1.90) \times 10^3$ | $(5.02 \pm 1.55) \times 10^3$ | $9.21 \pm 0.71$ |
| † | $(1.05 \pm 0.03) \times 10^7$ | 0.0292 | $68.6 \pm 9.8$ | $64.8 \pm 16.1$ | $(7.30 \pm 1.44) \times 10^3$ | $(8.72 \pm 2.05) \times 10^3$ | $(5.21 \pm 1.46) \times 10^3$ | $9.19 \pm 0.73$ |
| | $(1.05 \pm 0.03) \times 10^7$ | 0.0292 | $68.6 \pm 12.1$ | $64.6 \pm 16.2$ | $(7.28 \pm 1.42) \times 10^3$ | $(7.40 \pm 1.55) \times 10^3$ | $(4.87 \pm 1.58) \times 10^3$ | – |
| | $(1.25 \pm 0.03) \times 10^7$ | 0.0292 | $71.1 \pm 10.2$ | $68.3 \pm 15.2$ | $(7.64 \pm 1.43) \times 10^3$ | $(9.19 \pm 2.23) \times 10^3$ | $(5.53 \pm 1.58) \times 10^3$ | $9.93 \pm 0.73$ |
| | $(1.26 \pm 0.04) \times 10^7$ | 0.0292 | $77.0 \pm 14.7$ | $71.8 \pm 15.0$ | $(8.00 \pm 1.41) \times 10^3$ | $(8.35 \pm 1.77) \times 10^3$ | $(5.15 \pm 1.62) \times 10^3$ | $9.82 \pm 0.61$ |
| | $(1.27 \pm 0.03) \times 10^7$ | 0.0292 | $69.6 \pm 13.3$ | $67.5 \pm 18.9$ | $(7.68 \pm 1.64) \times 10^3$ | $(9.15 \pm 2.94) \times 10^3$ | $(5.80 \pm 1.73) \times 10^3$ | – |
| | $(1.66 \pm 0.04) \times 10^7$ | 0.0292 | $80.9 \pm 25.7$ | $74.5 \pm 19.0$ | $(8.47 \pm 1.94) \times 10^3$ | $(1.07 \pm 0.28) \times 10^4$ | $(6.23 \pm 1.84) \times 10^3$ | $11.0 \pm 0.8$ |
| | $(1.67 \pm 0.04) \times 10^7$ | 0.0292 | $83.5 \pm 11.8$ | $80.3 \pm 18.4$ | $(9.01 \pm 1.71) \times 10^3$ | $(1.04 \pm 0.30) \times 10^4$ | $(5.85 \pm 1.85) \times 10^3$ | $10.9 \pm 0.8$ |
| | $(1.73 \pm 0.04) \times 10^7$ | 0.0292 | $80.1 \pm 8.6$ | $80.3 \pm 20.4$ | $(9.08 \pm 1.80) \times 10^3$ | $(1.07 \pm 0.32) \times 10^4$ | $(6.33 \pm 1.90) \times 10^3$ | $12.2 \pm 1.0$ |
| | $(1.80 \pm 0.04) \times 10^7$ | 0.0291 | $82.9 \pm 10.0$ | $81.3 \pm 17.7$ | $(9.11 \pm 1.69) \times 10^3$ | $(8.95 \pm 2.77) \times 10^3$ | $(6.28 \pm 1.87) \times 10^3$ | – |
| | $(2.51 \pm 0.06) \times 10^7$ | 0.0292 | $93.9 \pm 13.3$ | $83.2 \pm 23.9$ | $(9.56 \pm 2.30) \times 10^3$ | $(1.29 \pm 0.34) \times 10^4$ | $(7.62 \pm 2.28) \times 10^3$ | $11.8 \pm 0.8$ |
| | $(2.53 \pm 0.06) \times 10^7$ | 0.0292 | $97.0 \pm 13.7$ | $93.1 \pm 22.8$ | $(1.05 \pm 0.21) \times 10^4$ | $(1.11 \pm 0.23) \times 10^4$ | $(7.40 \pm 2.25) \times 10^3$ | $12.1 \pm 0.7$ |
| | $(2.54 \pm 0.05) \times 10^7$ | 0.0292 | $101 \pm 22$ | $93.2 \pm 21.3$ | $(1.05 \pm 0.20) \times 10^4$ | $(1.24 \pm 0.42) \times 10^4$ | $(7.42 \pm 2.16) \times 10^3$ | $12.6 \pm 0.9$ |
| | $(2.55 \pm 0.06) \times 10^7$ | 0.0292 | $98.3 \pm 15.4$ | $96.8 \pm 20.6$ | $(1.08 \pm 0.20) \times 10^4$ | $(1.11 \pm 0.32) \times 10^4$ | $(7.18 \pm 2.21) \times 10^3$ | – |
| | $(3.32 \pm 0.09) \times 10^7$ | 0.0292 | $111 \pm 15$ | $105 \pm 29$ | $(1.21 \pm 0.29) \times 10^4$ | $(1.50 \pm 0.44) \times 10^4$ | $(8.36 \pm 2.36) \times 10^3$ | $12.5 \pm 0.7$ |
| | $(3.34 \pm 0.07) \times 10^7$ | 0.0292 | $105 \pm 16$ | $99.0 \pm 25.7$ | $(1.13 \pm 0.26) \times 10^4$ | $(1.43 \pm 0.45) \times 10^4$ | $(8.34 \pm 2.50) \times 10^3$ | $12.6 \pm 0.6$ |
| | $(3.34 \pm 0.07) \times 10^7$ | 0.0292 | $108 \pm 21$ | $103 \pm 27$ | $(1.17 \pm 0.24) \times 10^4$ | $(1.20 \pm 0.34) \times 10^4$ | $(8.34 \pm 2.49) \times 10^3$ | $14.2 \pm 0.9$ |
| | $(3.39 \pm 0.07) \times 10^7$ | 0.0292 | $106 \pm 13$ | $110 \pm 25$ | $(1.23 \pm 0.23) \times 10^4$ | $(1.44 \pm 0.46) \times 10^4$ | $(8.64 \pm 2.56) \times 10^3$ | $13.3 \pm 0.9$ |
| | $(4.82 \pm 0.10) \times 10^7$ | 0.0291 | $132 \pm 15$ | $125 \pm 30$ | $(1.41 \pm 0.28) \times 10^4$ | $(1.31 \pm 0.43) \times 10^4$ | $(9.50 \pm 2.82) \times 10^3$ | $14.4 \pm 0.7$ |
| | $(4.85 \pm 0.09) \times 10^7$ | 0.0290 | $130 \pm 27$ | $124 \pm 32$ | $(1.41 \pm 0.28) \times 10^4$ | $(1.58 \pm 0.55) \times 10^4$ | $(1.01 \pm 0.30) \times 10^4$ | $14.0 \pm 0.8$ |
| | $(5.11 \pm 0.10) \times 10^7$ | 0.0290 | $131 \pm 17$ | $124 \pm 30$ | $(1.41 \pm 0.29) \times 10^4$ | $(1.68 \pm 0.53) \times 10^4$ | $(9.97 \pm 3.04) \times 10^3$ | $14.5 \pm 0.8$ |
| | $(5.28 \pm 0.10) \times 10^7$ | 0.0290 | $129 \pm 16$ | $129 \pm 32$ | $(1.47 \pm 0.30) \times 10^4$ | $(1.70 \pm 0.55) \times 10^4$ | $(1.02 \pm 0.33) \times 10^4$ | $14.7 \pm 0.8$ |
| | $(5.81 \pm 0.11) \times 10^7$ | 0.0291 | $137 \pm 32$ | $134 \pm 32$ | $(1.51 \pm 0.30) \times 10^4$ | $(1.71 \pm 0.62) \times 10^4$ | $(1.10 \pm 0.32) \times 10^4$ | $14.5 \pm 0.7$ |
| | $(5.82 \pm 0.12) \times 10^7$ | 0.0281 | $137 \pm 20$ | $129 \pm 33$ | $(1.52 \pm 0.32) \times 10^4$ | $(1.43 \pm 0.43) \times 10^4$ | $(1.09 \pm 0.32) \times 10^4$ | $15.3 \pm 0.8$ |
| | $(5.89 \pm 0.13) \times 10^7$ | 0.0281 | $136 \pm 23$ | $133 \pm 36$ | $(1.57 \pm 0.33) \times 10^4$ | $(1.79 \pm 0.61) \times 10^4$ | $(1.10 \pm 0.34) \times 10^4$ | $15.1 \pm 0.9$ |
| † | $(5.93 \pm 0.13) \times 10^7$ | 0.0280 | $134 \pm 26$ | $124 \pm 32$ | $(1.47 \pm 0.33) \times 10^4$ | $(1.46 \pm 0.46) \times 10^4$ | $(1.13 \pm 0.33) \times 10^4$ | $14.8 \pm 0.8$ |
